# Supplementary material for: Re-examining the boundary conditions in modelling SAW-driven acoustofluidic streaming
Source: arXiv:2511.12585 source file (2025-11-16)
Supplement: Supplementary file 1 [file Supplemental_Material.pdf]

# Supplemental Material: Revisiting the Boundary Conditions in Modelling SAW-Driven Acoustofluidic Streaming

Qinran Wei, Suyu Ding, Yang Zhao, Yuanpeng Ma, Dachuan Sang, Dong Zhang, and Xiasheng Guo

*Key Laboratory of Modern Acoustics (MOE), School of Physics,*

*Collaborative Innovation Center of Advanced Microstructures,*

*Nanjing University, Nanjing 210093, China*

(Dated: November 16, 2025)

## A. Implementation of the Reynolds Stress Method (RSM) in Two-Dimension

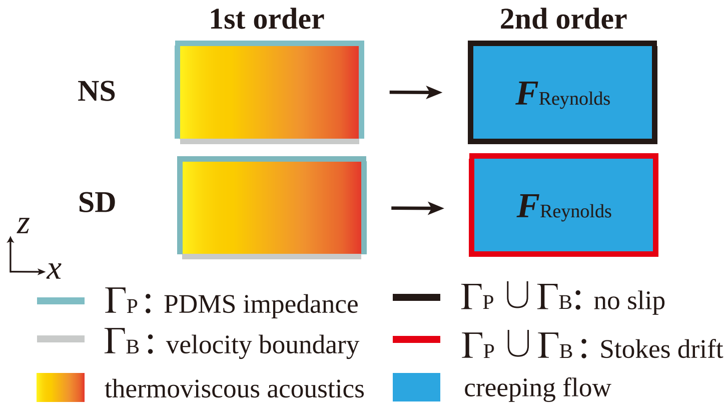


FIG. S1. Two-dimensional schematic of the RSM model setup.

The two-dimensional schematic of the RSM method with different second-order boundary conditions is illustrated in Fig. S1.

In COMSOL Multiphysics, the first-order governing equations are implemented using the "Thermoviscous Acoustics, Frequency Domain" interface. The boundary $\Gamma_{\mathrm{B}}$ (piezoelectric substrate) is assigned a "Velocity" condition defined by the acoustic vibration superposition formula (Eq. (10) in the main text), while the boundary $\Gamma_{\mathrm{P}}$ (PDMS wall) is modelled using an "Impedance" condition.

The second-order governing equations are solved via the "Single Phase Flow" interface. Boundaries $\Gamma_{\mathrm{P}} \cup \Gamma_{\mathrm{B}}$ are specified either as a no-slip "Wall" (NS–RSM) or assigned a Stokes slip velocity in the "Wall Movement" section (SD–RSM). The Reynolds stress is incorporated as a body force, and the mass source term is implemented via a "Weak Contribution" node. A "Global Constraint" is applied to ensure solution uniqueness. All second-order equations are solved using a "Stationary" study.

For simulations without thermoviscous corrections, all boundaries $\Gamma_{\mathrm{P}} \cup \Gamma_{\mathrm{B}}$ are set to "isothermal". When thermoviscous corrections are included, $\Gamma_{\mathrm{P}}$ is set to "adiabatic" and $\Gamma_{\mathrm{B}}$ remains "isothermal".

## B. Mesh Convergence Analysis and Discretization Criteria

A standing surface acoustic wave (SSAW) device with wavelength $\lambda_{\mathrm{s}} = 200$ µm, channel width $W = \lambda_{\mathrm{s}}$, and height $H = 0.5\lambda_{\mathrm{v}}$ is used for convergence analysis. A boundary layer region of thickness $10\delta_{\mathrm{v}}$ is defined along all fluid domain boundaries. A quadrilateral mapped mesh is used

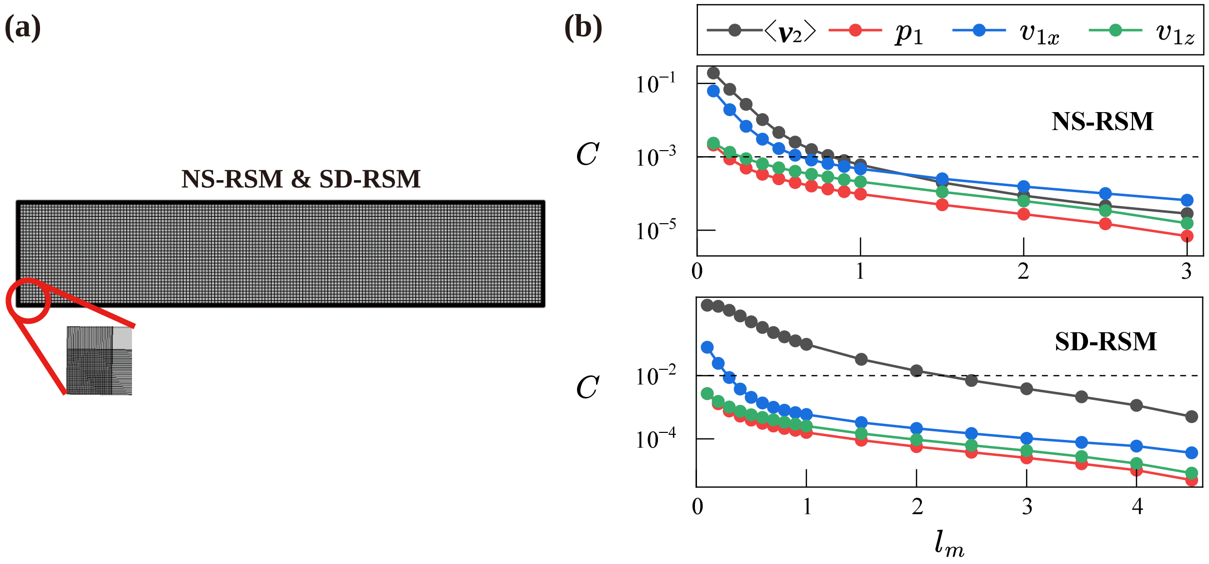


FIG. S2. (a) Mesh design for the RSM simulation. (b) Convergence factor $C$ for physical fields $p_1$, $v_{1x}$, $v_{1z}$, and $\langle \boldsymbol{v}_2 \rangle$ as a function of the boundary layer mesh factor $l_m$.

within this layer, and a free quadrilateral mesh in the bulk region. The maximum element size within the boundary layer is $\delta_\mathrm{v}/l_m$, where $l_m$ is the boundary mesh refinement factor. In the bulk, the maximum element size is limited to $b_m\delta_\mathrm{v}$, where $b_m$ is the bulk mesh factor.

The convergence factor $C$ is defined as [1, 2]:

$$C(g) = \sqrt{\frac{\iint (g - g_\mathrm{ref})^2\, \mathrm{d}x\mathrm{d}z}{\iint g_\mathrm{ref}^2 \mathrm{d}x\mathrm{d}z}}, \tag{S1}$$

where $g(x, z)$ denotes a physical field distribution for a given mesh, and $g_\mathrm{ref}$ is the reference solution obtained under a highly refined mesh.

Results of the boundary layer mesh convergence analysis are shown in Fig. S2. For the NS condition, $g_\mathrm{ref}$ is obtained with $b_m = 5$, $l_m = 3.5$; for the SD condition, $g_\mathrm{ref}$ uses $b_m = 5$, $l_m = 5$. To ensure $C < 0.001$ for all fields, we select $l_m = 1.5$ for the NS condition and $l_m = 3.5$ for the SD condition. The slower convergence under the SD condition is attributed to the Stokes slip boundary.

Bulk mesh convergence results are shown in Fig. S3. The reference solution for the NS condition uses $b_m = 3$, $l_m = 2$; for the SD condition, $b_m = 3$, $l_m = 3.5$. A bulk factor $b_m$ between 3 and 10 ensures $C < 0.0025$ in both cases. All two-dimensional simulations in the main text adhere to these mesh settings.

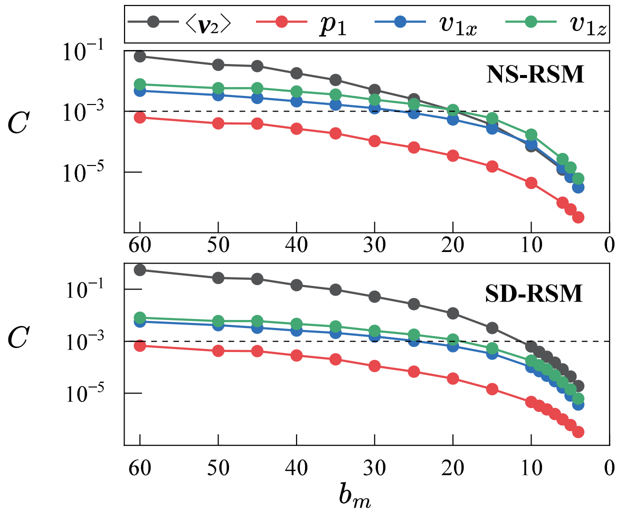


FIG. S3. Convergence factor $C$ for $p_1$, $v_{1x}$, $v_{1z}$, and $\langle \boldsymbol{v}_2 \rangle$ as a function of the bulk mesh factor $b_m$.

### C. Material Parameters used in Simulation

| | | |
|---|---|---|
| **Water, $\boldsymbol{T}$=25°C** | | |
| Density[3] | $\rho_0$ | 998 kg m$^{-3}$ |
| Speed of Sound [3] | $c_0$ | 1495 m s$^{-1}$ |
| Dynamic viscosity [3] | $\mu$ | 0.893 mPa s |
| Bulk viscosity[1] | $\mu^{\mathrm{B}}$ | 2.47 mPa s |
| Specific heat capacity [3] | $C_p$ | 4183 J kg$^{-1}$ K$^{-1}$ |
| Thermal conductivity [3] | $k_{\mathrm{th}}$ | 0.603 W m$^{-1}$ K$^{-1}$ |
| Thermal expansion coefficient [3] | $\alpha_0$ | $2.97 \times 10^{-4}$ K$^{-1}$ |
| Specific heat capacity ratio [3] | $\gamma$ | 1.014 |
| | $(1/\mu)\,\partial\mu/\partial T$ | $-2.57 \times 10^{-2}$ K$^{-1}$ |
| Thermodynamic derivatives | $(1/\mu)\,\partial\mu/\partial\rho$ | $-3.472 \times 10^{-4}$ kg$^{-1}$ m$^3$ |
| | $\left(1/\mu^{\mathrm{B}}\right)\partial\mu^{\mathrm{B}}/\partial T$ | $-2.584 \times 10^{-2}$ K$^{-1}$ |
| **Polydimethylsiloxane (PDMS)** | | |
| Density[4] | $\rho_{\mathrm{P}}$ | 1030.5 kg m$^{-3}$ |
| Longitudinal wave speed[2] | $c_{\mathrm{P}}$ | 1030 m s$^{-1}$ |
| **128° $\boldsymbol{Y}$-$\boldsymbol{X}$ $\mathbf{LiNbO_3}$** | | |
| Density | $\rho_{\mathrm{LN}}$ | 4700 kg m$^{-3}$ |
| Speed of Sound[1] | $c_{\mathrm{LN}}$ | 3994 m s$^{-1}$ |

## D. Simplified Simulation Method Employing the NS Condition

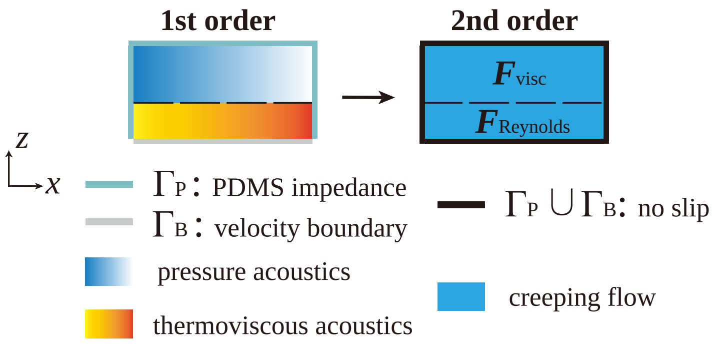


FIG. S4. Two-dimensional schematic of the simplified model under the NS condition.

### 1. *COMSOL Model Configuration*

A schematic of the model setup is illustrated in Fig. S4. The governing equations within the thermoviscous layer remain identical to those used in the RSM method. Outside this layer, the first-order acoustic field is described by the effective Helmholtz equation,

$$\nabla^2 p_1 + \frac{\omega^2}{c_{\rm eff}^2} p_1 = 0, \tag{S2}$$

where $c_{\rm eff} = c_0 \left(1 + \mathrm{i}\omega \frac{\frac{4}{3}\mu + \mu_{\rm B}}{\rho_0 c_0^2}\right)^{1/2}$ is the complex effective speed of sound.

The second-order equations outside the thermoviscous layer are

$$\begin{aligned} \rho_0 \nabla \cdot \langle \boldsymbol{v}_2 \rangle &= 0, \\ -\nabla \langle p_2 \rangle + \mu\beta \nabla(\nabla \cdot \langle \boldsymbol{v}_2 \rangle) + \mu \nabla^2 \langle \boldsymbol{v}_2 \rangle &= -\boldsymbol{F}_{\rm visc}, \end{aligned} \tag{S3}$$

with the viscous acoustic body force defined as $\boldsymbol{F}_{\rm visc} = \frac{(\beta+1)\mu\omega^2}{\rho_0 c_0^4} \boldsymbol{I}$.

For the simplified model under the NS condition, the first-order equations inside the thermoviscous layer are solved using the "Thermoviscous Acoustics, Frequency Domain" interface. The boundary $\Gamma_{\rm B}$ (substrate) uses a "Velocity" condition with the superposition formula (Eq. (10)) from the main text, and $\Gamma_{\rm P}$ (PDMS) uses an "Impedance" condition. The interface between the thermoviscous layer and the outer domain employs the "Acoustic–Thermoviscous Acoustic Boundary" condition. The outer domain is modelled using the "Pressure Acoustics, Frequency Domain" interface.

Second-order flow is solved via the "Single Phase Flow" interface. Source terms inside the thermoviscous layer match those in RSM; outside, $\boldsymbol{F}_{\text{visc}}$ is applied as a body force. A "Global Constraint" ensures the uniqueness of the second-order pressure. All domain boundaries are set to no-slip. A "Stationary" study is used to solve the system.

In two-dimensional simulations, mapped meshes are used within the thermoviscous layer and free quad meshes elsewhere. The maximum element size in the bulk is $10\delta_{\text{v}}$ for Devices A and B, and $15\delta_{\text{v}}$ for Device C. Within the thermoviscous layer, the maximum element size is $\delta_{\text{v}}$, and the layer thickness is set to $5.3\delta_{\text{v}}$.

In three-dimensional simulations, free triangular and swept meshes are used. A symmetry condition is applied at $y = 0$, and an impedance condition (matched to water) at $y = L$. For all devices, the free triangular mesh has a maximum size of $\lambda_{\text{f}}/4$. The number of swept elements in the outer region is 20 for Devices A and C, and 10 for Device B. The thermoviscous layer thickness is uniformly set to $5\delta_{\text{v}}$.

### *2. Validation of the Simplified Method*

Figure S5 compares two-dimensional velocity distributions in the $x$–$z$ cross-section between the full RSM and the simplified method for all three experimental devices. The results confirm that the simplified method effectively captures the acoustic streaming patterns that the full model produces under the NS condition.

### *3. Optimal Thermoviscous Layer Thickness*

To quantify the agreement between the simplified method and full RSM for varying thermoviscous layer thicknesses $t_m\delta_{\text{v}}$, we use the model difference factor [5]

$$D(f_1, f_2) = \sqrt{\frac{\iint (f_1 - f_2)^2 \mathrm{d}x\mathrm{d}z}{\iint f_2^2 \mathrm{d}x\mathrm{d}z}}, \tag{S4}$$

where $f_1$ is the field from the simplified model and $f_2$ the reference from RSM.

First, investigate the relationship between optimal thickness and surface acoustic wave (SAW) wavelength for devices with $\lambda_{\text{s}} = 600, 300, 200, 150$ μm, fixed $W = \lambda_{\text{s}}$, and $H = 0.5\lambda_{\text{v}}$. A coarse scan of $t_m \in [1, 14]$ (the left panel of Fig. S6 shows the minimum $D(f_1)$ occurs for $t_m \in (4, 7)$. A refined scan (the right panel of Fig. S6(b)) shows the optimum lies in $5.2 \sim 5.4\delta_{\text{v}}$, with a slight increase for longer wavelengths.

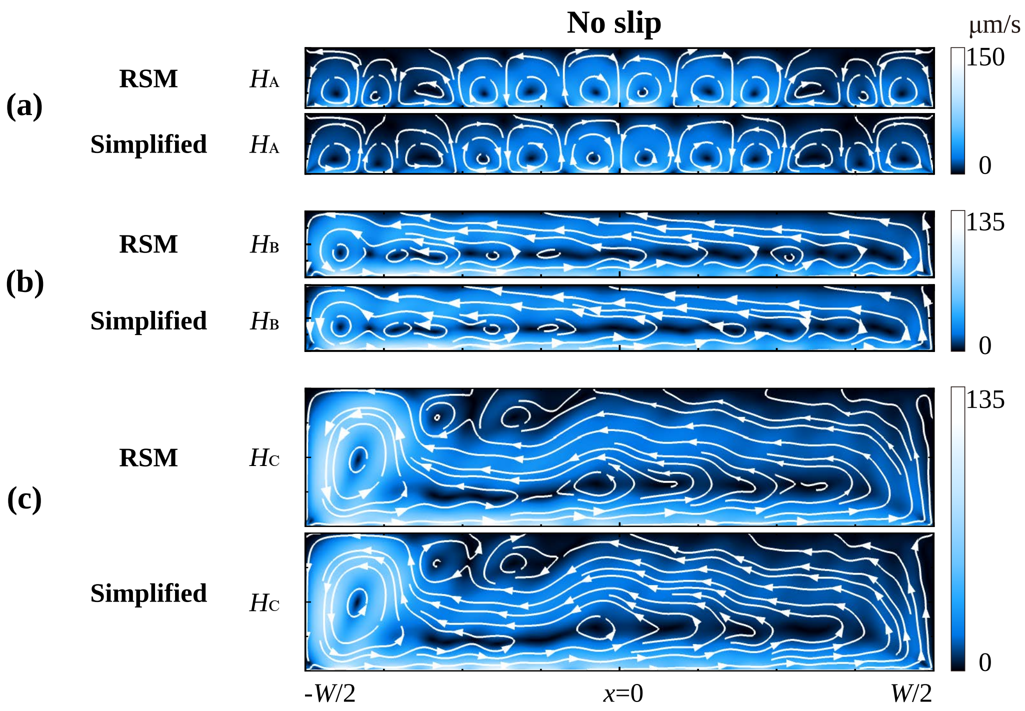


FIG. S5. Comparison of Lagrangian velocity $\boldsymbol{v}^{\mathrm{L}}$ from the simplified method and the full RSM under the NS condition. (a) Device A: $H_{\mathrm{A}} = 56$ μm, $W = 600$ μm, $\lambda_{\mathrm{s}} = 200$ μm, $\xi_1 = 0.3$ nm, $\Delta\phi = \pi$. (b) Device B: $H_{\mathrm{B}} = 62$ μm, $W = 600$ μm, $\lambda_{\mathrm{s}} = 80$ μm, $\xi_1 = 0.3$ nm. (c) Device C: $H_{\mathrm{C}} = 131$ μm, $W = 600$ μm, $\lambda_{\mathrm{s}} = 80$ μm, $\xi_1 = 0.3$ nm.

Then, fix $\lambda_{\mathrm{s}} = 200$ μm and vary $W = \lambda_{\mathrm{s}}, 2\lambda_{\mathrm{s}}, 3\lambda_{\mathrm{s}}$ and $H$ in steps of $\lambda_{\mathrm{v}}/4$. The optimal thickness (Table S1) oscillates between $4.7 \sim 5.4\delta_{\mathrm{v}}$ periodically with $H$: for $H = (2n-1)\lambda_{\mathrm{v}}/4$, $T_{\mathrm{optimal}} \approx 4.7 \sim 4.9\delta_{\mathrm{v}}$; for $H = n\lambda_{\mathrm{v}}/2$, $T_{\mathrm{optimal}} \approx 5.2 \sim 5.4\delta_{\mathrm{v}}$. This behaviour may relate to channel geometry and mesh structure within the thermoviscous layer.

TABLE S1. Optimal layer thicknesses for devices with different geometric dimensions. $\lambda_{\mathrm{s}} = 200$ μm.

| $T_{\mathrm{optimal}}/\delta_{\mathrm{v}}$ ; $H/\lambda_{\mathrm{v}}$ ; $W$ | 0.25 | 0.5 | 0.75 | 1 | 1.25 | 1.5 | 1.75 | 2 | 2.25 | 2.5 | 2.75 | 3 | 3.25 | 3.5 | 3.75 |
|---|---|---|---|---|---|---|---|---|---|---|---|---|---|---|---|
| $\lambda_{\mathrm{s}}$ | 4.7 | 5.3 | 4.7 | 5.3 | 4.8 | 5.3 | 4.8 | 5.3 | 4.8 | 5.2 | 4.8 | 5.2 | 4.9 | 5.2 | 4.9 |
| $2\lambda_{\mathrm{s}}$ | 4.7 | 5.3 | 4.7 | 5.4 | 4.8 | 5.3 | 4.8 | 5.4 | 4.8 | 5.3 | 4.8 | 5.3 | 4.8 | 5.3 | 4.8 |
| $3\lambda_{\mathrm{s}}$ | 4.7 | 5.3 | 4.7 | 5.3 | 4.7 | 5.4 | 4.7 | 5.3 | 4.8 | 5.3 | 4.8 | 5.3 | 4.8 | 5.3 | 4.8 |

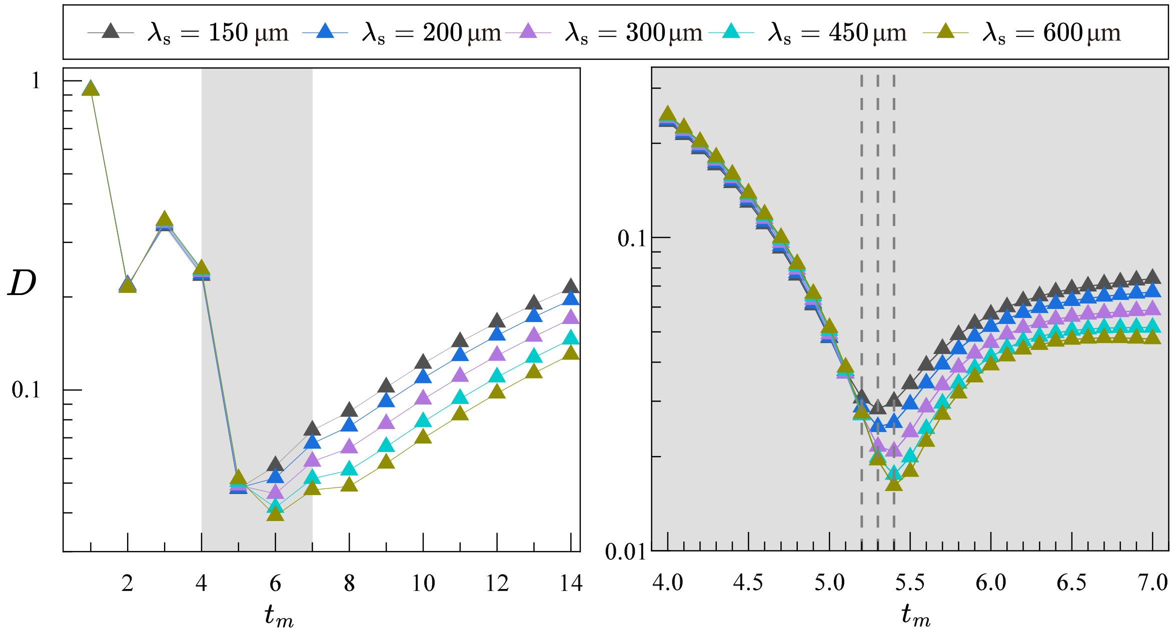


FIG. S6. Model difference factor $D$ for $\langle \boldsymbol{v}_2 \rangle$ as a function of the thermoviscous layer thickness factor $t_m$ for devices of different wavelengths. Channel dimensions: $w = 1$, $h = 0.5$. Left: coarse scan; right: fine scan (logarithmic vertical scale).

### E. The Simplified Method with the SD Condition

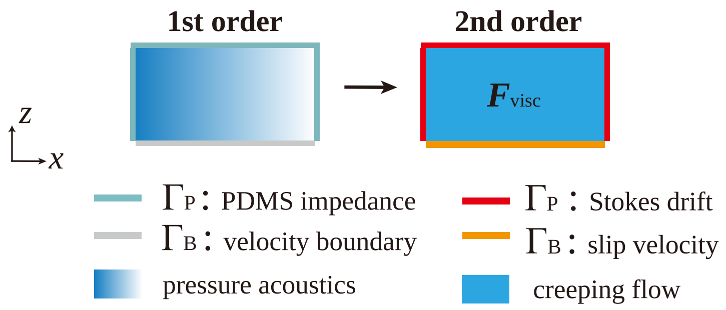


FIG. S7. Two-dimensional schematic of the simplified model under the SD condition.

#### 1. *Model Configuration in COMSOL*

The model setup is illustrated in Fig. S7. The first- and second-order governing equations are given by Eq. (S2) and Eq. (S3), respectively. The slip velocity (Eq. (S2)) is implemented following the equivalent formulation of Bach & Bruus [6].

The first-order equations are solved using the "Pressure Acoustics, Frequency Domain" interface. Boundary $\Gamma_{\mathrm{B}}$ is assigned a "Velocity" condition, and $\Gamma_{\mathrm{P}}$ an "Impedance" condition.

Second-order flow is computed via the "Single Phase Flow" interface. The Stokes drift term is prescribed in the "Wall Movement" section of the "Wall" boundary condition. The viscous body force $\boldsymbol{F}_{\mathrm{visc}}$ is applied throughout the domain. A "Stationary" study is used to solve the system.

In two-dimensional simulations, a free quadrilateral mesh is used with a maximum element size of $10\delta_{\mathrm{v}}$ for Devices A and B, and $15\delta_{\mathrm{v}}$ for Device C.

In three-dimensional modelling, free triangular and swept meshes are employed. A symmetry condition is applied at $y = 0$, and an impedance condition (matched to water) at $y = L$. The maximum element size of the triangular mesh is $\lambda_{\mathrm{f}}/4$ for all devices. The number of swept elements is 20 for Devices A and C, and 10 for Device B.

#### 2. *Validation of the Simplified Method*

Figure S8 compares the two-dimensional velocity distributions in the $x$–$z$ cross-section between the full RSM and the simplified method for all three experimental devices. The results demonstrate

that the simplified method effectively reproduces the acoustic streaming patterns under the SD condition.

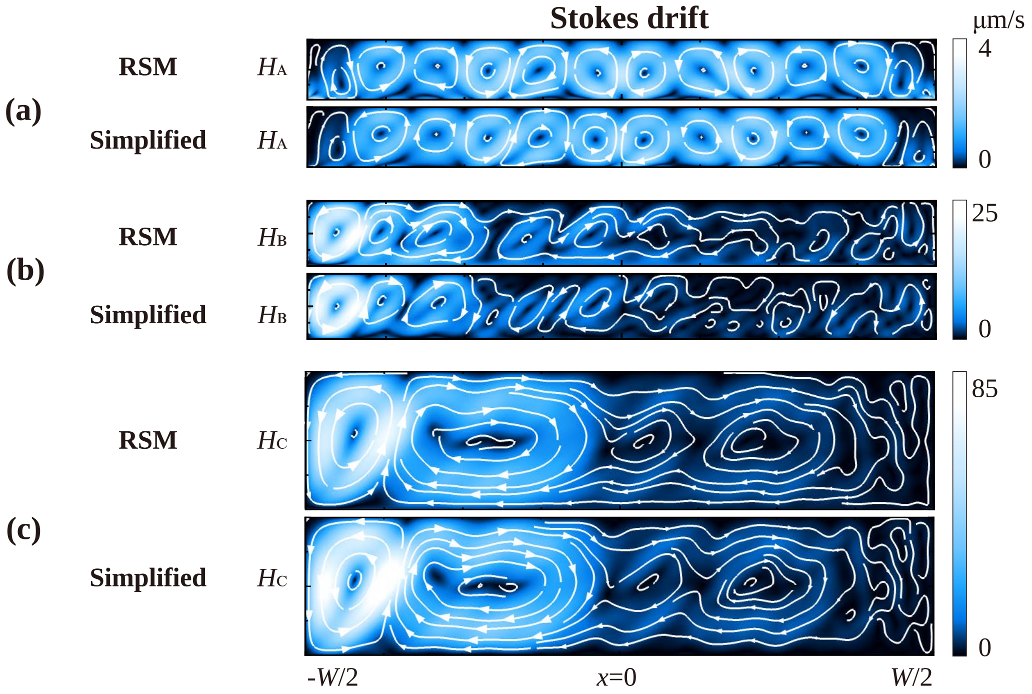


FIG. S8. Comparison of Lagrangian velocity $\boldsymbol{v}^{\mathrm{L}}$ from the simplified method and the full RSM under the SD condition. Device parameters are the same as in Fig. S5.

### F. Convergence of NS and SD Solutions under Lobe Streaming Dominance

When the channel height satisfies $H > W \cot \theta_{\mathrm{R}}$, lobe streaming becomes the dominant flow structure. Under this condition, the amplitudes of boundary-driven streaming and other vortices are significantly reduced compared to the lobe streaming. As illustrated in Fig. S9, the numerical results obtained using the NS and SD conditions converge, indicating that the influence of the Stokes drift term becomes negligible.

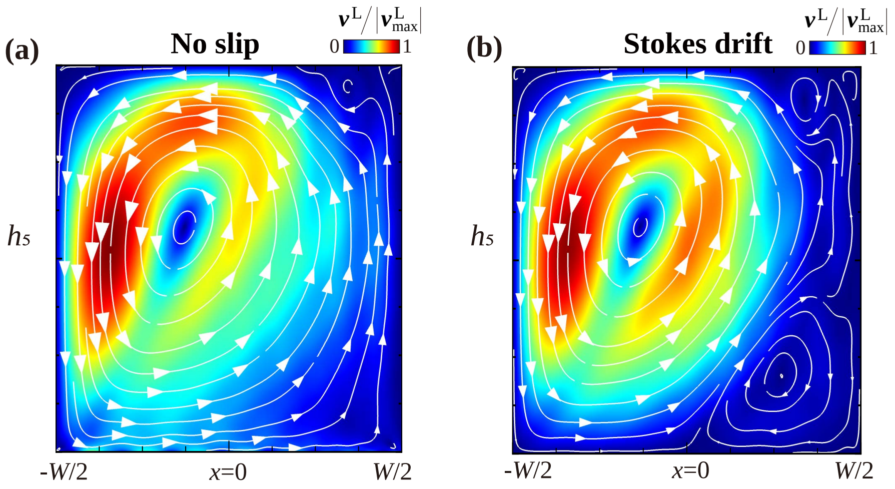


FIG. S9. Acoustic streaming patterns generated by a TSAW propagating in the $+x$ direction under (a) NS and (b) SD conditions for $h_5 = 11$. Parameters: $w = 4$, $\lambda_{\mathrm{s}} = 200$ μm, $\lambda_{\mathrm{v}} = 80.7$ μm, $\xi_1 = 1$ nm.

### G. Calculation of the Normalized Substrate Displacement Distribution

The normalized displacement distribution $\hat{\xi}(y)$ is computed from the amplitude distribution of the piezoelectric substrate using the angular spectrum method for plane waves [7]. A pair of interdigital transducers (IDTs) is modelled as a finite-length line source, which excites SAWs on the anisotropic piezoelectric substrate described by

$$\xi_0(X,Y) = \int_{-\infty}^{+\infty} \frac{\sin\left(k_Y A/2\right) e^{-\mathrm{i}(k_X X + k_Y Y)}}{\pi k_Y} \mathrm{d}k_Y, \quad (X \geq 0), \tag{S5}$$

where $X = x + d$, $Y = y$, and $A$ is the aperture. The wavenumbers $k_X$ and $k_Y$ are related through the slowness surface of the substrate.

For IDTs consisting of $N$ finger pairs, the total vibration field is obtained by superposing contributions from multiple equivalent line sources with appropriate time delays [8]

$$\xi(X,Y) = \sum_{i=0}^{2N-1} (-1)^i \cdot \xi_0\left(X + \tfrac{1}{2}k_\mathrm{s}\lambda_\mathrm{s}, Y\right). \tag{S6}$$

The normalized displacement amplitude along the $y$-direction at the channel wall is then given by

$$\hat{\xi}(y) = \left.\frac{\xi(X,Y)}{|\xi(X,Y)|_{\max}}\right|_{X=d}. \tag{S7}$$

### H. Implementation of Thermoviscous Corrections in the RSM Framework

Following the approach of Nama *et al.* [9] for thermoviscous corrections in the arbitrary Lagrangian–Eulerian (ALE) method, we incorporate analogous modifications into both the NS- and SD-RSM formulations. The first-order temperature boundary conditions are set as “adiabatic” on $\Gamma_\mathrm{P}$ and “isothermal” on $\Gamma_\mathrm{B}$.

In addition to the Reynolds stress term $\boldsymbol{F}_\mathrm{Reynolds}$, the total body force now includes two viscosity-dependent terms,

$$\boldsymbol{F} = \boldsymbol{F}_\mathrm{Reynolds} + \nabla \cdot \langle \mu_\mathrm{B1}(\nabla \cdot \boldsymbol{v}_1)\boldsymbol{E}\rangle + \nabla \cdot \left\langle \mu_1 \left(\nabla \boldsymbol{v}_1 + \nabla \boldsymbol{v}_1^T\right)\right\rangle, \tag{S8}$$

where $\boldsymbol{E}$ is the identity matrix. The first-order viscosity coefficients are defined as

$$\mu_1 = \frac{\partial \mu}{\partial \rho}\rho_1 + \frac{\partial \mu}{\partial T}T_1, \qquad \mu_\mathrm{B1} = \frac{\partial \mu^\mathrm{B}}{\partial T}T_1 + \frac{\partial \mu^\mathrm{B}}{\partial \rho}\rho_1.$$

Note that the density dependence of the bulk viscosity $\mu^\mathrm{B}$ for water is not well-documented in the literature.

If thermoviscous corrections are not applied, all boundaries are set to an “isothermal” condition.

## I. Acoustic Pressure Calibration via Particle Tracking in SSAW Devices

The acoustic pressure in an SSAW device is determined by balancing the $x$-components of the acoustic radiation force $\boldsymbol{F}^{\mathrm{rad}}$ and the hydrodynamic drag force $\boldsymbol{F}^{\mathrm{drag}}$ acting on a polystyrene (PS) particle [10]. The SSAW field consists of a standing wave along $x$ and a travelling wave component along $z$.

The $x$-component of the acoustic radiation force is given by

$$F_x^{\mathrm{rad}} = -4\pi\Phi k_{\mathrm{s}} a^3 E_{\mathrm{ac}} \sin\left(2k_{\mathrm{s}}x + \Delta\phi\right), \tag{S9}$$

where $E_{\mathrm{ac}} = |p_1|^2/(4\rho_0 c_0^2)$ is the acoustic energy density, $\Delta\phi$ is the phase difference between counter-propagating waves, and $\Phi = f_1/3 + \mathrm{Re}(f_2)(\sin^2\theta_{\mathrm{R}} - 0.5)$ is the acoustic contrast factor. Here, $f_1$ and $f_2$ denote the monopole and dipole scattering coefficients, respectively.

For a PS particle with radius $a = 2.5$ µm in a channel of height $H = 56$ µm, the distance to the nearest wall is $l = 16$ µm. The wall correction factor is

$$\chi \approx \left(1 - \frac{9a}{16l} + \frac{a^3}{8l^3} - \frac{45a^4}{256l^4} - \frac{a^5}{16l^5}\right)^{-1} = 1.0959. \tag{S10}$$

The corresponding drag force is then

$$F_x^{\mathrm{drag}} = -6\pi\chi\mu a\frac{\mathrm{d}x}{\mathrm{d}t}. \tag{S11}$$

Balancing the two forces yields the particle trajectory

$$x(t) = \frac{1}{k_{\mathrm{s}}}\arctan\left\{\tan\left[k_{\mathrm{s}}(x(0) - x_{\mathrm{N}})\right]\exp\left(-\frac{4k_{\mathrm{s}}^2\Phi a^2}{3\mu}E_{\mathrm{ac}}t\right)\right\} + x_{\mathrm{N}}, \tag{S12}$$

where $x(0)$ is the initial position and $x_{\mathrm{N}}$ is the nearest pressure node. Values of $x_{\mathrm{N}}$ and $E_{\mathrm{ac}}$ are obtained via least-squares fitting in MATLAB (see Fig. S11), from which the pressure amplitude $|p_1|$ is derived.

The measured pressure corresponds to the peak of the $z$-averaged pressure $\overline{|p_1|}$ (Fig. S12) [10]. For a pressure antinode at the channel center, the average of five peak values in the central region ($-200$ µm $< x <$ 200 µm) is used. The normalized displacement amplitude $\hat{\xi}(y)$ is shown in Fig. S10; PIV measurements were conducted in the central aperture region (green area).

A fitting curve between $\overline{|p_1|}$ and displacement amplitude $\xi_1$ was obtained from parametric simulations (right panel of Fig. S13). Experimentally measured pressure amplitudes at various voltages (left panel of Fig. S13) were used to infer $\xi_1$ for streaming simulations.

The maximum $x$-component of Lagrangian velocity $\boldsymbol{v}^{\mathrm{L}}$ in the region $-200$ µm $< x <$ 200 µm, $0 < z < 15$ µm was compared to PIV results at $z = 5$ µm (see main text). When

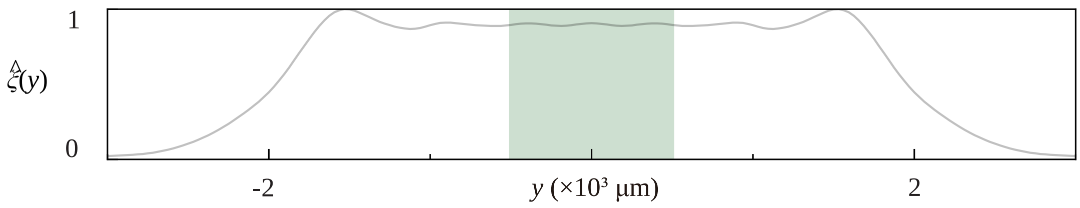


FIG. S10. Normalized displacement amplitude $\hat{\xi}(y)$ along the $y$-direction for the SSAW device (Device A). The green region indicates the measurement area used in experiments.

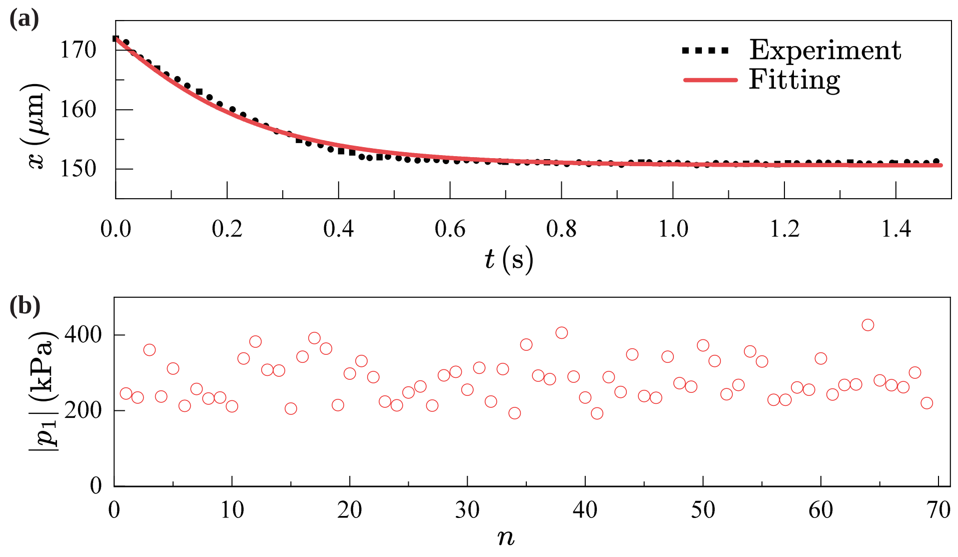


FIG. S11. (a) Least-squares fit (solid line) and experimentally measured particle trajectory (dots) in the $x$-direction at $V = 70$ mV. (b) Acoustic pressure profile derived from particle tracking at $V = 70$ mV. $n$ represents the tracking number of the particle.

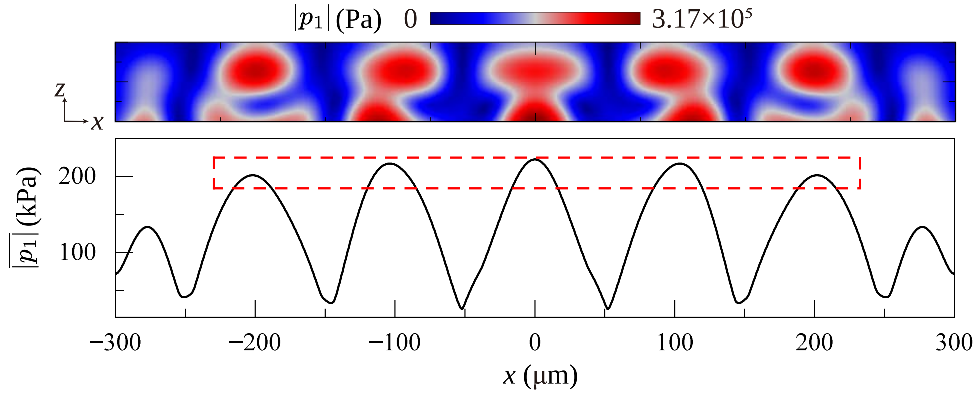


FIG. S12. Acoustic pressure distribution $|p_1|$ in the $x$–$z$ cross-section, and the corresponding $z$-averaged pressure $\overline{|p_1|}$ for displacement amplitude $\xi_1 = 0.5$ nm. Device A parameters with $\Delta\phi = \pi$.

the channel center is a pressure node, vortex directions from NS-condition simulations oppose experimental observations, whereas SD-condition results agree closely (Fig. S14).

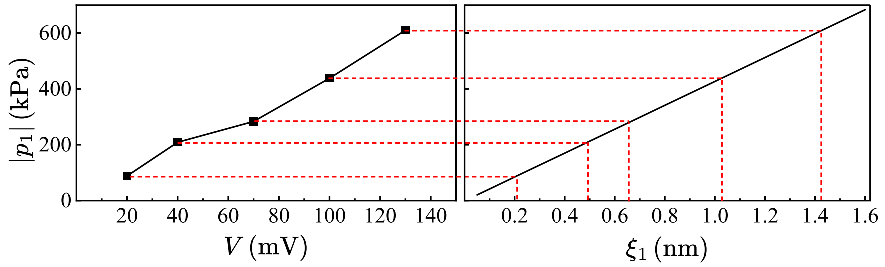


FIG. S13. Left: Acoustic pressure amplitudes measured via particle tracking at different driving voltages. Right: Mean peak values of $\overline{|p_1|}$ as a function of displacement amplitude $\xi_1$.

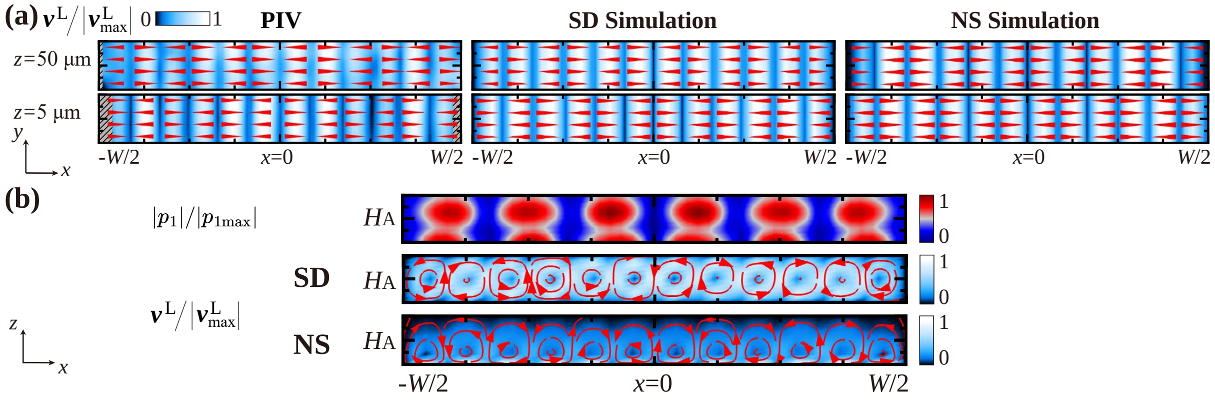


FIG. S14. (a) Comparison of the $x$-component of velocity in the $x$–$y$ plane between PIV measurements and simulations at $z = 50$ μm (1) and $z = 5$ μm (2), when the channel center is a pressure node. (b) Normalized pressure $|p_1|$ and Lagrangian velocity $\boldsymbol{v}^{\mathrm{L}}$ in the $x$–$z$ cross-section ($y = 0$) under SD and NS conditions. Parameters: $\lambda_{\mathrm{s}} = 200$ μm, $W = 600$ μm, $H_{\mathrm{A}} = 56$ μm, $\Delta\phi = 0$.

### J. Characteristics of Stokes Drift in SAW-Driven Acoustofluidic Streaming

#### 1. *Relation between Stokes Drift and Acoustic Intensity in the Inviscid Limit*

In the absence of viscosity, for a plane traveling wave $p_1 = |p_1|e^{\mathrm{i}\omega t - \mathrm{i}\boldsymbol{k}\cdot\boldsymbol{r}}$, we have $\nabla p_1 = -\mathrm{i}\boldsymbol{k}p_1$. From the first-order momentum equation $\rho_0 \frac{\partial \boldsymbol{v}_1}{\partial t} = -\nabla p_1$, it follows that $\boldsymbol{v}_1 = -\dfrac{1}{\mathrm{i}\omega\rho_0}\nabla p_1 = \dfrac{p_1}{\omega\rho_0}\boldsymbol{k}$. For any time-harmonic fields $A_1(\boldsymbol{r},t)$, $B_1(\boldsymbol{r},t)$ (with factor $e^{\mathrm{i}\omega t}$), the time average satisfies $\langle A_1(\boldsymbol{r},t)B_1(\boldsymbol{r},t)\rangle = \frac{1}{2}\mathrm{Re}\left[A_1(\boldsymbol{r})^* B_1(\boldsymbol{r})\right]$.

The acoustic intensity is $\boldsymbol{I} = \langle p_1\boldsymbol{v}_1\rangle = \dfrac{|p_1|^2}{2\omega\rho_0}\boldsymbol{k}$, and the Stokes drift velocity $\boldsymbol{v}^{\mathrm{SD}}$ is proportional to $\boldsymbol{I}$:

$$\boldsymbol{v}^{\mathrm{SD}} = \langle \frac{1}{\mathrm{i}\omega}\boldsymbol{v}_1 \cdot \nabla \boldsymbol{v}_1 \rangle \tag{S13a}$$

$$= \frac{1}{2}\mathrm{Re}\left[\left(\frac{1}{\mathrm{i}\omega}\boldsymbol{v}_1\right)^* \cdot \nabla \boldsymbol{v}_1\right] \tag{S13b}$$

$$= \frac{1}{2\omega}\mathrm{Re}\left[\left(\frac{p_1}{\omega\rho_0}\boldsymbol{k}e^{-\mathrm{i}\frac{\pi}{2}}\right)^* \cdot \nabla\left(\frac{p_1}{\omega\rho_0}\boldsymbol{k}\right)\right] \tag{S13c}$$

$$= \frac{1}{2\omega^3\rho_0^2}\mathrm{Re}\left(p_1^* e^{\mathrm{i}\frac{\pi}{2}}\boldsymbol{k}\cdot\nabla p_1\boldsymbol{k}\right) \tag{S13d}$$

$$= \frac{|\boldsymbol{k}|^2}{2\omega^3\rho_0^2}\mathrm{Re}\left(\mathrm{i}p_1^*\hat{\boldsymbol{k}}\cdot\nabla p_1\hat{\boldsymbol{k}}\right) \tag{S13e}$$

$$= \frac{|\boldsymbol{k}|^2}{2\omega^3\rho_0^2}\mathrm{Re}\left[\mathrm{i}p_1^*\left(-\mathrm{i}\boldsymbol{k}\right)p_1\right] \tag{S13f}$$

$$= \frac{|p_1|^2}{4\omega\left(\rho_0 c_0\right)^2}\boldsymbol{k} \tag{S13g}$$

$$= \frac{\boldsymbol{I}}{2\rho_0 c_0^2}. \tag{S13h}$$

Here, $\hat{\boldsymbol{k}} = \dfrac{\boldsymbol{k}}{|\boldsymbol{k}|}$ is the direction vector corresponding to the wave vector of the travelling wave. The above derivation uses $\hat{\boldsymbol{k}}\cdot\nabla\left(e^{-\mathrm{i}\boldsymbol{k}\cdot\boldsymbol{r}}\hat{\boldsymbol{k}}\right) = \left(-\mathrm{i}\boldsymbol{k}\right)e^{-\mathrm{i}\boldsymbol{k}\cdot\boldsymbol{r}}$.

A pure standing wave, being a superposition of counter-propagating waves, has zero net intensity ($\boldsymbol{I} = 0$) and hence zero Stokes drift. This explains why $\boldsymbol{v}^{\mathrm{SD}}$ aligns with $\boldsymbol{I}$ in regions far from boundaries in SAW devices.

#### 2. *Stokes Drift in a Tall SSAW Channel*

To quantify differences between Eulerian and Lagrangian velocities, we use the model difference factor $D$ from Eq. (S4), with $f_1 = \boldsymbol{v}^{\mathrm{E}}$ and $f_2 = \boldsymbol{v}^{\mathrm{L}}$. Figure S15 shows flow distributions and $D$ as a function of $H/\lambda_{\mathrm{v}}$ for an SSAW device with $H = 6\lambda_{\mathrm{v}}$. The Eulerian and Lagrangian velocities

are similar in the bulk but differ significantly within the bottom boundary layer, confirming that the Stokes drift primarily influences near-wall boundary-driven streaming.

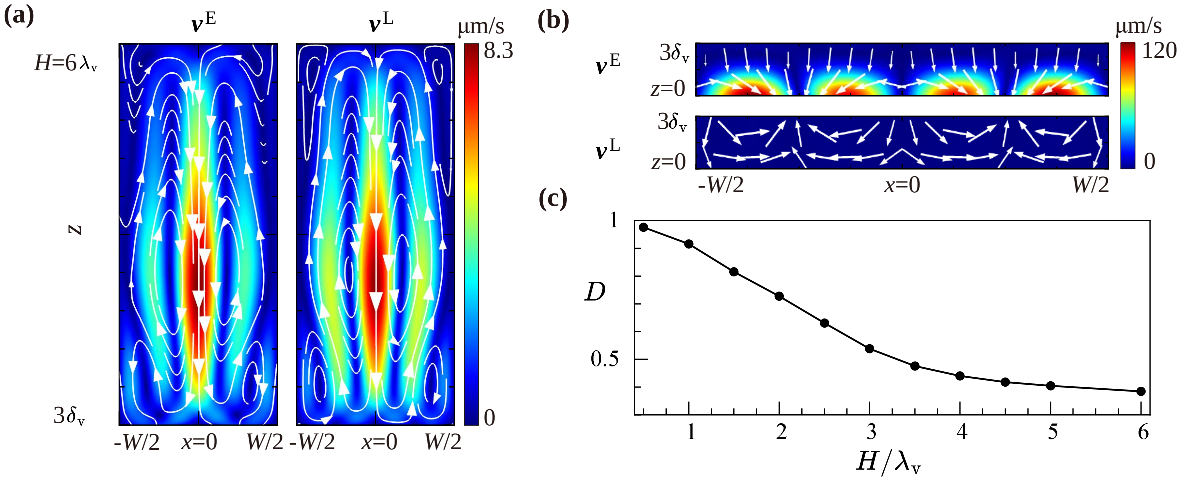


FIG. S15. (a) Distributions of Eulerian velocity $\boldsymbol{v}^{\mathrm{E}}$ and Lagrangian velocity $\boldsymbol{v}^{\mathrm{L}}$ for an SSAW device with $h = 6$, shown in the bulk region and (b) within the boundary layer. (c) Model difference factor $D$ of $\boldsymbol{v}^{\mathrm{L}}$ relative to $\boldsymbol{v}^{\mathrm{E}}$ as a function of the normalized channel height $H/\lambda_{\mathrm{v}}$. Parameters: $w = 1$, $\lambda_{\mathrm{s}} = 200$ μm, $\lambda_{\mathrm{v}} = 80.7$ μm, $\xi_1 = 0.3$ nm, $\Delta\phi = 0$.

### *3. Stokes Drift Distribution in TSAW Devices*

Figure S16 shows the height profiles of $x$-averaged $|\boldsymbol{v}^{\mathrm{E}}|$, $|\boldsymbol{v}^{\mathrm{L}}|$, and $|\boldsymbol{v}^{\mathrm{SD}}|$, and their spatial distributions for two TSAW devices with different channel heights.

Within the boundary layer, shear stress causes $\boldsymbol{v}^{\mathrm{SD}}$ to be dominated by its $x$-component. Outside the boundary layer, $\boldsymbol{v}^{\mathrm{SD}}$ aligns with the oblique incidence direction of the acoustic wave, consistent with the direction of $\boldsymbol{I}$ (Fig. S16(b)). In both cases, the $x$-component of $\boldsymbol{v}^{\mathrm{SD}}$ decays by nearly three orders of magnitude within $z = 0.1$–$1$ μm, while the $z$-component remains nearly constant.

Near the wall, $|\boldsymbol{v}^{\mathrm{SD}}|$ and $|\boldsymbol{v}^{\mathrm{E}}|$ are comparable in magnitude but opposite in direction, resulting in a much smaller $|\boldsymbol{v}^{\mathrm{L}}|$. In the bulk, due to partial cancellation between $v_z^{\mathrm{SD}}$ and $v_z^{\mathrm{E}}$, the $x$-averaged $|v_z^{\mathrm{L}}|$ is smaller than $|v_z^{\mathrm{E}}|$ in lower channel ($h = 0.75$). In higher channel ($h = 6$), the effect of acoustic attenuation makes $|v_z^{\mathrm{L}}|$ and $|v_z^{\mathrm{E}}|$ comparable at $z > 20$ μm.

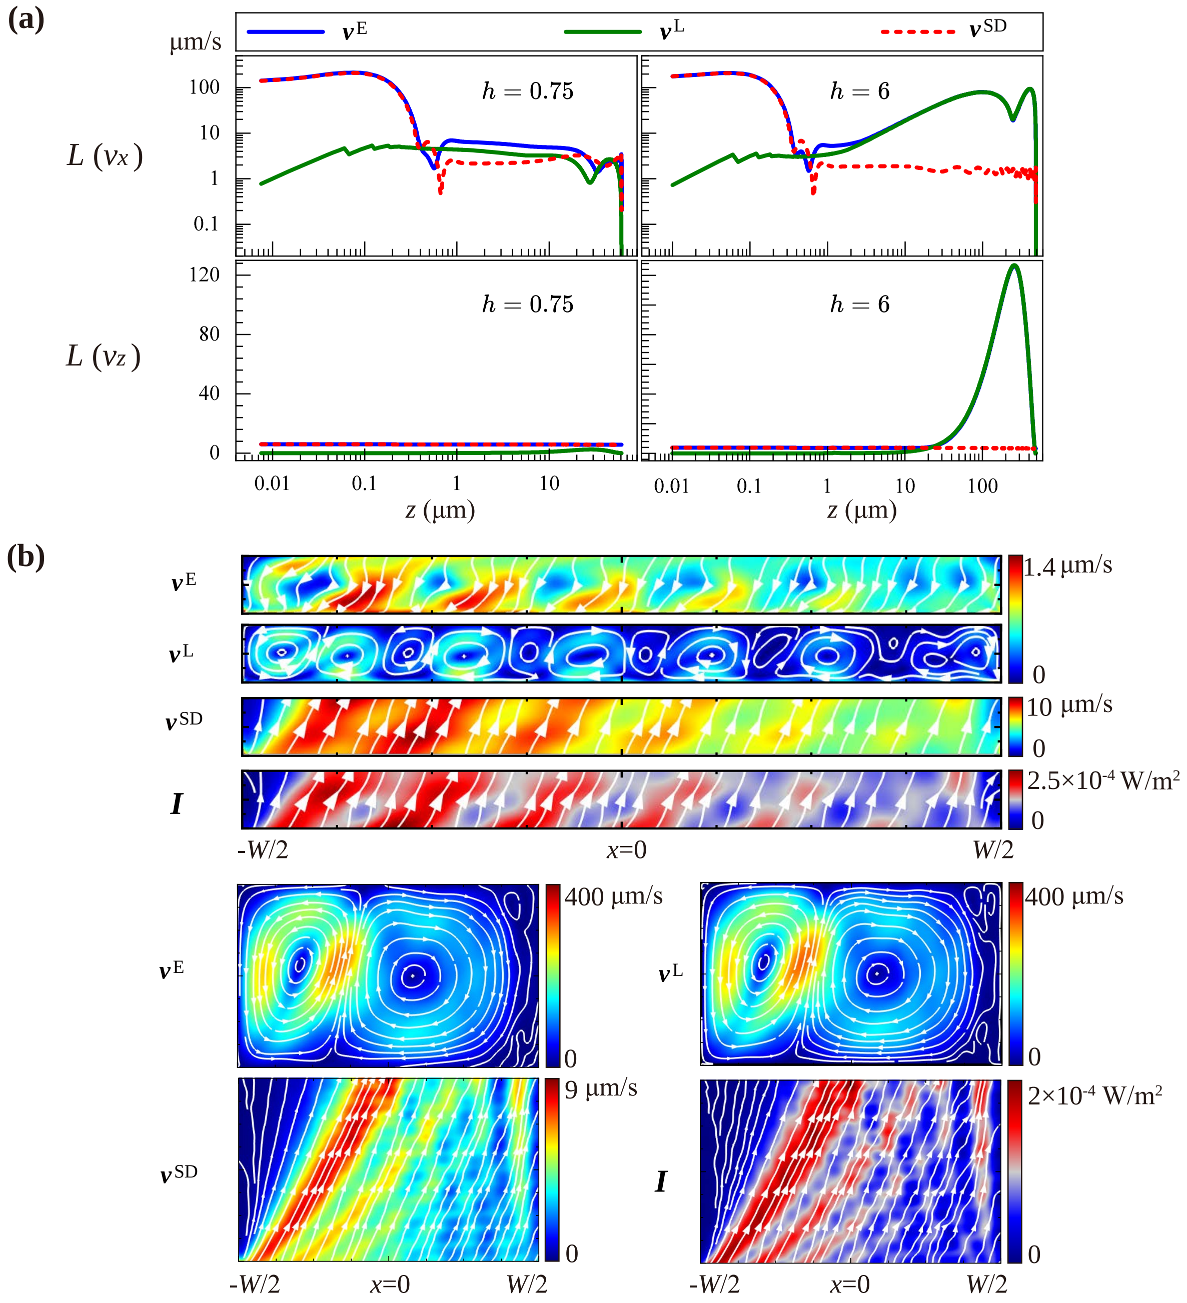


FIG. S16. For TSAW devices with two channel heights: (a) $x$-averaged profiles of $|\boldsymbol{v}^{\mathrm{E}}|$, $|\boldsymbol{v}^{\mathrm{L}}|$, and $|\boldsymbol{v}^{\mathrm{SD}}|$ versus height $z$; (b) spatial distributions of $\boldsymbol{v}^{\mathrm{E}}$, $\boldsymbol{v}^{\mathrm{L}}$, $\boldsymbol{v}^{\mathrm{SD}}$, and acoustic intensity $\boldsymbol{I}$. Color indicates magnitude; arrows show vector direction. Parameters: $w = 4$, $\lambda_{\mathrm{s}} = 200$ μm, $\lambda_{\mathrm{v}} = 80.7$ μm, $\xi_1 = 1$ nm.

### K. Formulas for Slip Velocity

Slip velocity by Bach & Bruus[6] (corresponding to the SD condition):

$$\begin{aligned}u_{\mathrm{slip}} = -\frac{1}{2\omega}\mathrm{Re}\Big\{&1.5\,(1+\mathrm{i})\,U_1\frac{\mathrm{d}U_1^*}{\mathrm{d}t_1}\\&+(0.5+\mathrm{i})\,V_1\frac{\mathrm{d}U_1^*}{\mathrm{d}t_2}+(1+0.5\mathrm{i})\,U_1\frac{\mathrm{d}V_1^*}{\mathrm{d}t_2}\\&+\mathrm{i}\left(\frac{\mathrm{d}v_{1t_1}}{\mathrm{d}t_1}+\frac{\mathrm{d}v_{1t_2}}{\mathrm{d}t_2}-\frac{\mathrm{d}v_{1n}}{\mathrm{d}n}\right)U_1^*+2\mathrm{i}\frac{\mathrm{d}V_1}{\mathrm{d}t_1}V_1^*\Big\},\end{aligned} \tag{S14a}$$

$$\begin{aligned}v_{\mathrm{slip}} = -\frac{1}{2\omega}\mathrm{Re}\Big\{&1.5\,(1+\mathrm{i})\,V_1\frac{\mathrm{d}V_1^*}{\mathrm{d}t_2}\\&+(0.5+\mathrm{i})\,U_1\frac{\mathrm{d}V_1^*}{\mathrm{d}t_1}+(1+0.5\mathrm{i})\,V_1\frac{\mathrm{d}U_1^*}{\mathrm{d}t_1}\\&+\mathrm{i}\left(\frac{\mathrm{d}v_{1t_2}}{\mathrm{d}t_2}+\frac{\mathrm{d}v_{1t_1}}{\mathrm{d}t_1}-\frac{\mathrm{d}v_{1n}}{\mathrm{d}n}\right)V_1^*+2\mathrm{i}\frac{\mathrm{d}U_1}{\mathrm{d}t_2}U_1^*\Big\}.\end{aligned} \tag{S14b}$$

Slip velocity by Lee & Wang[11] (corresponding to the NS condition):

$$\begin{aligned}u_{\mathrm{slip}}^{\mathrm{LVM}} = -\frac{1}{4\omega}\mathrm{Re}\Big\{&U_1\frac{\mathrm{d}U_1^*}{\mathrm{d}t_1}+V_1\frac{\mathrm{d}U_1^*}{\mathrm{d}t_2}\\&+(2+\mathrm{i})\,U_1^*\nabla\cdot\boldsymbol{U}_1-U_1^*\,(2+3\mathrm{i})\,\frac{\mathrm{d}W_1}{\mathrm{d}n}\Big\},\end{aligned} \tag{S15a}$$

$$\begin{aligned}v_{\mathrm{slip}}^{\mathrm{LVM}} = -\frac{1}{4\omega}\mathrm{Re}\Big\{&V_1\frac{\mathrm{d}V_1^*}{\mathrm{d}t_2}+U_1\frac{\mathrm{d}V_1^*}{\mathrm{d}t_1}\\&+(2+\mathrm{i})\,V_1^*\nabla\cdot\boldsymbol{U}_1-U_1^*\,(2+3\mathrm{i})\,\frac{\mathrm{d}W_1}{\mathrm{d}n}\Big\}.\end{aligned} \tag{S15b}$$

At the solid–liquid interface, let $\boldsymbol{n} = (n_x, n_y, n_z)$ denote the unit normal vector, and $\boldsymbol{t_1} = (t_{1x}, t_{1y}, t_{1z})$, $\boldsymbol{t_2} = (t_{2x}, t_{2y}, t_{2z})$ the orthogonal unit tangent vectors. The slip velocity expression, originally formulated in the boundary coordinate system $(t_1, t_2, n)$, must be transformed into the global Cartesian basis $(x, y, z)$ for numerical implementation. In both the 2D and 3D models considered here, the boundary coordinate system aligns with the global Cartesian system, so no additional transformation is required.

The components of the vector $\boldsymbol{U}_1 = (U_1, V_1, W_1)$ are defined as

$$\begin{aligned}U_1 &= v_{1t_1} - u_{1t_1},\\ V_1 &= v_{1t_2} - u_{1t_2},\\ W_1 &= v_{1n},\end{aligned} \tag{S16}$$

where $v_{1t_1}, v_{1t_2}, v_{1n}$ are the tangential and normal components of the irrotational acoustic velocity field $\boldsymbol{v}_1$, and $u_{1t_1}, u_{1t_2}$ are the tangential components of the solid vibration velocity $\boldsymbol{u}_1$.

### L. Equations for ALE method

For the ALE method, the first-order governing equations are consistent with those of the RSM. The second-order equations are

$$\nabla \cdot \boldsymbol{v}^{\mathrm{L}} = 0, \quad \nabla \cdot \langle \boldsymbol{P}_2 \rangle = 0, \tag{S17}$$

where

$$\begin{aligned}
\langle \boldsymbol{P}_2 \rangle = & -\langle p_2 \rangle \boldsymbol{E} + \mu \left[ \nabla \boldsymbol{v}^{\mathrm{L}} + \left( \nabla \boldsymbol{v}^{\mathrm{L}} \right)^T \right] + \frac{1}{2} c_0^2 \rho_0 \left( \frac{1}{\mathrm{i}\omega} \right)^2 \langle (\nabla \cdot \boldsymbol{v}_1)^2 - \nabla \boldsymbol{v}_1^T : \nabla \boldsymbol{v}_1 \rangle \boldsymbol{E} \\
& + \mu^{\mathrm{B}} \left( \frac{1}{\mathrm{i}\omega} \right) \langle (\nabla \cdot \boldsymbol{v}_1)^2 - \nabla \boldsymbol{v}_1^T : \nabla \boldsymbol{v}_1 \rangle \boldsymbol{E} + \mu \langle \nabla \cdot \boldsymbol{v}_1 \left( \nabla \boldsymbol{v}_1 \nabla \boldsymbol{v}_1^T \right) - \nabla \boldsymbol{v}_1 \nabla \boldsymbol{v}_1 - \nabla \boldsymbol{v}_1^T \nabla \boldsymbol{v}_1^T \rangle \\
& - \left( \frac{1}{\mathrm{i}\omega} \right) \langle \left[ c_0^2 \rho_0 \left( \nabla \cdot \boldsymbol{v}_1 \right) \boldsymbol{E} + \mu \left( \nabla \boldsymbol{v}_1 + \nabla \boldsymbol{v}_1^T \right) + \mu^{\mathrm{B}} \left( \nabla \cdot \boldsymbol{v}_1 \right) \boldsymbol{E} \right] \nabla \boldsymbol{v}_1^T \rangle \\
& + \langle \mu_1^{\mathrm{B}} \left( \nabla \cdot \boldsymbol{v}_1 \right) \boldsymbol{E} + \mu_1 \left( \nabla \boldsymbol{v}_1 + \nabla \boldsymbol{v}_1^T \right) \rangle .
\end{aligned} \tag{S18}$$

Equations above are implemented through the "Weak Form" interface in COMSOL.

**Supplemental Videos**

Video S1: Experimental recordings and PIV measurements of streaming patterns in the SSAW device, and particle trajectories used for acoustic pressure calibration.

Video S2: Experimental recordings and PIV results showing peripheral and lobe streaming vortices in the TSAW device.

---


[1] N. Nama, R. Barnkob, Z. Mao, C. J. Kähler, F. Costanzo, and T. J. Huang, Numerical study of acoustophoretic motion of particles in a PDMS microchannel driven by surface acoustic waves, Lab Chip **15**, 2700 (2015).

[2] N. Skov and H. Bruus, Modeling of Microdevices for SAW-Based Acoustophoresis — A Study of Boundary Conditions, Micromachines **7**, 182 (2016).

[3] P. B. Muller, R. Barnkob, M. J. H. Jensen, and H. Bruus, A numerical study of microparticle acoustophoresis driven by acoustic radiation forces and streaming-induced drag forces, Lab Chip **12**, 4617 (2012).

[4] G. Xu, Z. Ni, X. Chen, J. Tu, X. Guo, H. Bruus, and D. Zhang, Acoustic Characterization of Polydimethylsiloxane for Microscale Acoustofluidics, Phys. Rev. Appl. **13**, 054069 (2020).

[5] C. Chen, S. P. Zhang, Z. Mao, N. Nama, Y. Gu, P.-H. Huang, Y. Jing, X. Guo, F. Costanzo, and T. J. Huang, Three-dimensional numerical simulation and experimental investigation of boundary-driven streaming in surface acoustic wave microfluidics, Lab Chip **18**, 3645 (2018).

[6] J. S. Bach and H. Bruus, Theory of pressure acoustics with viscous boundary layers and streaming in curved elastic cavities, J. Acoust. Soc. Am. **144**, 766 (2018).

[7] M. Tan and C. Flory, Fast Computation of SAW Diffraction by Asymptotic Techniques, IEEE Trans. Ultrason. Ferroelectr. Freq. Control **34**, 93 (1987).

[8] Y. Zhang, J. Huang, and X. Guo, Field nonuniformity of limited-aperture planar SAWs and its implications for designing SSAW acoustofluidics, J. Micromech. Microeng. **31**, 094001 (2021).

[9] R. Barnkob, N. Nama, L. Ren, T. J. Huang, F. Costanzo, and C. J. Kähler, Acoustically Driven Fluid and Particle Motion in Confined and Leaky Systems, Phys. Rev. Appl. **9**, 014027 (2018).

[10] Z. Liu, H. Zheng, Q. Wei, Z. Wang, Y. Zhang, D. Zhang, and X. Guo, A look-up table protocol for calibrating standing SAW acoustofluidics, Microfluid. Nanofluid. **28**, 36 (2024).

[11] C. P. Lee and T. G. Wang, Near-boundary streaming around a small sphere due to two orthogonal standing waves, J. Acoust. Soc. Am. **85**, 1081 (1989).
